# Supplementary material for: Cross-Domain Video Anomaly Detection without Target Domain Adaptation
Source: arXiv:2212.07010 source file (2022-12-14)
Supplement: Supplementary file 1 [file supp_amount_of_TI_data.tex]

\begin{wrapfigure}{r}{7.8cm}
    \vspace*{-1\baselineskip}
    \centering
    \begin{subfigure}[t]{0.245\textwidth}
        \raggedright
        \input{plots/amount_hmdb}
        \caption{HMDB}
        \label{fig:amount_hmdb}
    \end{subfigure}%
    ~
    \begin{subfigure}[t]{0.245\textwidth}
        \raggedright
        \input{plots/amount_ucf101}
        \caption{UCF101}
        \label{fig:amount_ucf101}
    \end{subfigure}%
    \caption[Impact of amount of TI data on \zvad.]{\textbf{Impact of amount of TI data on} \zvad. }
    \label{fig:supp_amount_of_TI_data}
\end{wrapfigure}
