# Supplementary material for: Cross-Domain Video Anomaly Detection without Target Domain Adaptation
Source: arXiv:2212.07010 source file (2022-12-14)
Supplement: Supplementary file 2 [file supp_background_subtraction_methods.tex]

\begin{table}[t]
\resizebox{0.415\columnwidth}{!}{%
\begin{tabular}{cccccc}
\toprule
& &  & \multicolumn{3}{c}{\textbf{VAD Testing Data}} \\
 \cmidrule(l){4-6} 
\multirow{-2}{*}{\textbf{VAD Training Data}} &\multirow{-2}{*}{\textbf{TI Data}} &\multirow{-2}{*}{\textbf{Method}} &\textbf{Ped1} &\textbf{Ped2} &\textbf{Ave} \\
\midrule
SHT &N/A & NLAPnet \cite{roy2021predicting} (paper) & 71.60 & \textbf{95.90} & 74.70  \\
SHT &N/A & OC-AE \cite{ionescu2019object} (paper) & 74.40 & 90.30 & 78.80  \\
SHT &N/A & BA-AE \cite{georgescu2020background} (paper) & -- & 95.70 & 81.00  \\
\rowcolor{red!10}
SHT &N/A &\zvado  &\textbf{76.14} &{95.78} &82.28 \\
\rowcolor{red!10}
SHT &HMDB &\zvado &75.62 &95.74 &\textbf{83.19} \\
\rowcolor{red!10}
SHT &UCF101 &\zvado &75.41 &\underline{95.80} &82.25 \\
\rowcolor{red!10}
SHT &Jester &\zvado &\underline{75.93} &95.62 &\underline{82.49} \\
\bottomrule
\end{tabular}%
}
\caption[Comparison with background-subtraction based xVAD methods.]{\textbf{Comparison with background-subtraction based xVAD methods.} Source is SHT}
\label{tab:bg_method_exp}
\end{table}
